# Supplementary material for: Advances in Land Surface Model-based Forecasting: A comparative study of LSTM, Gradient Boosting, and Feedforward Neural Network Models as prognostic state emulators
Source: arXiv:2407.16463 source file (2024-07-23)

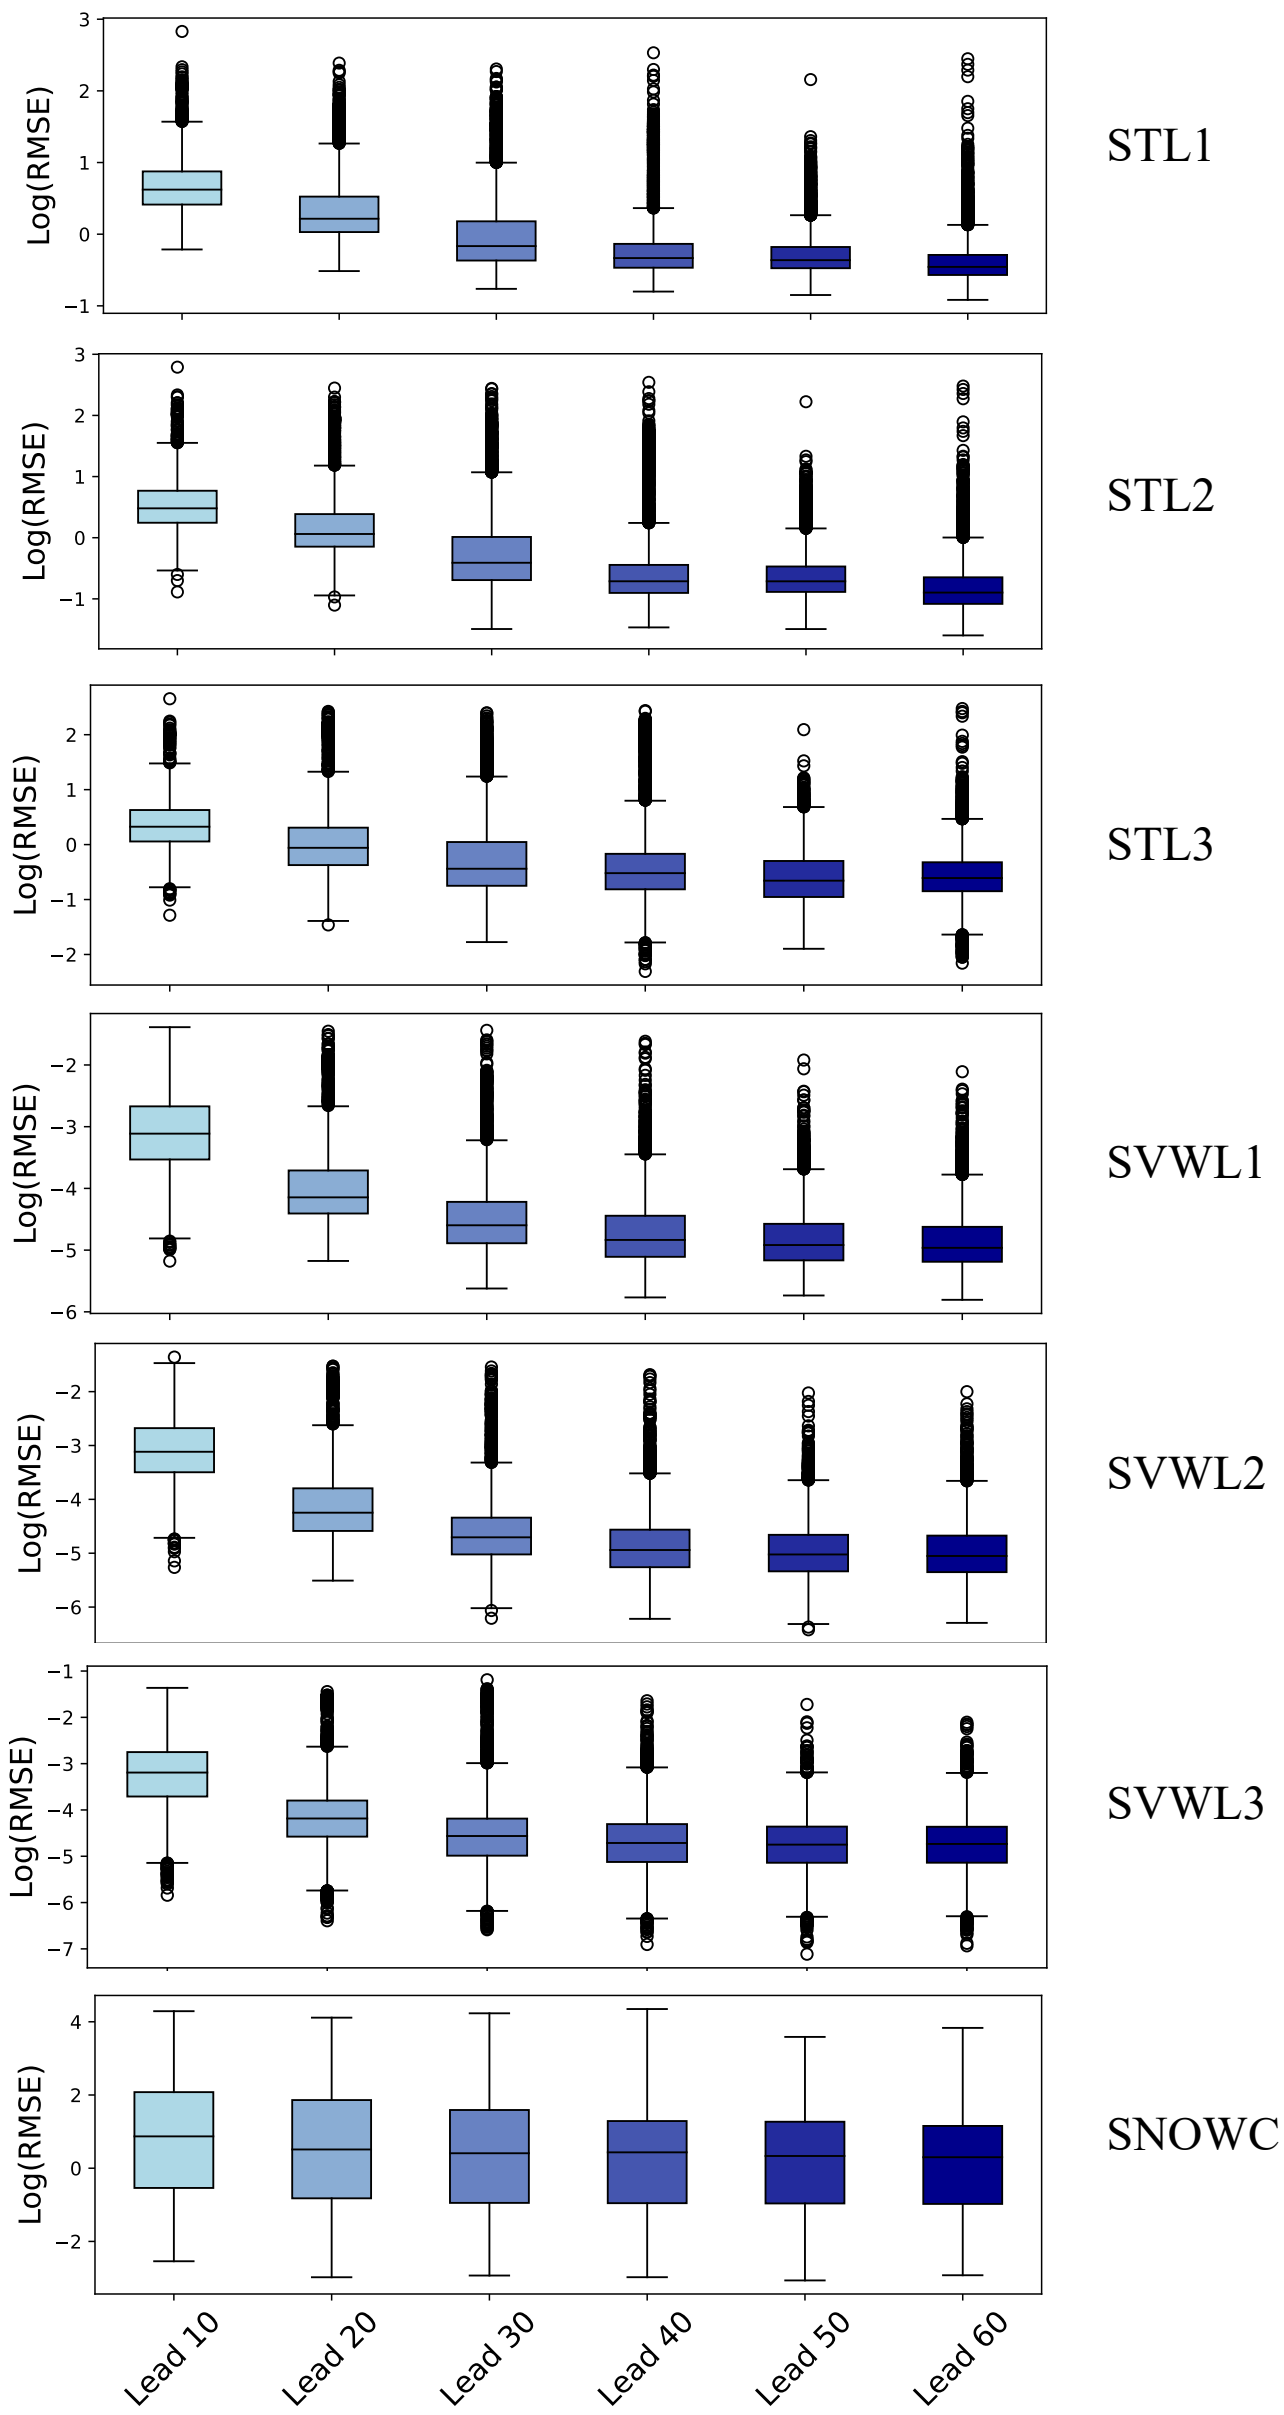

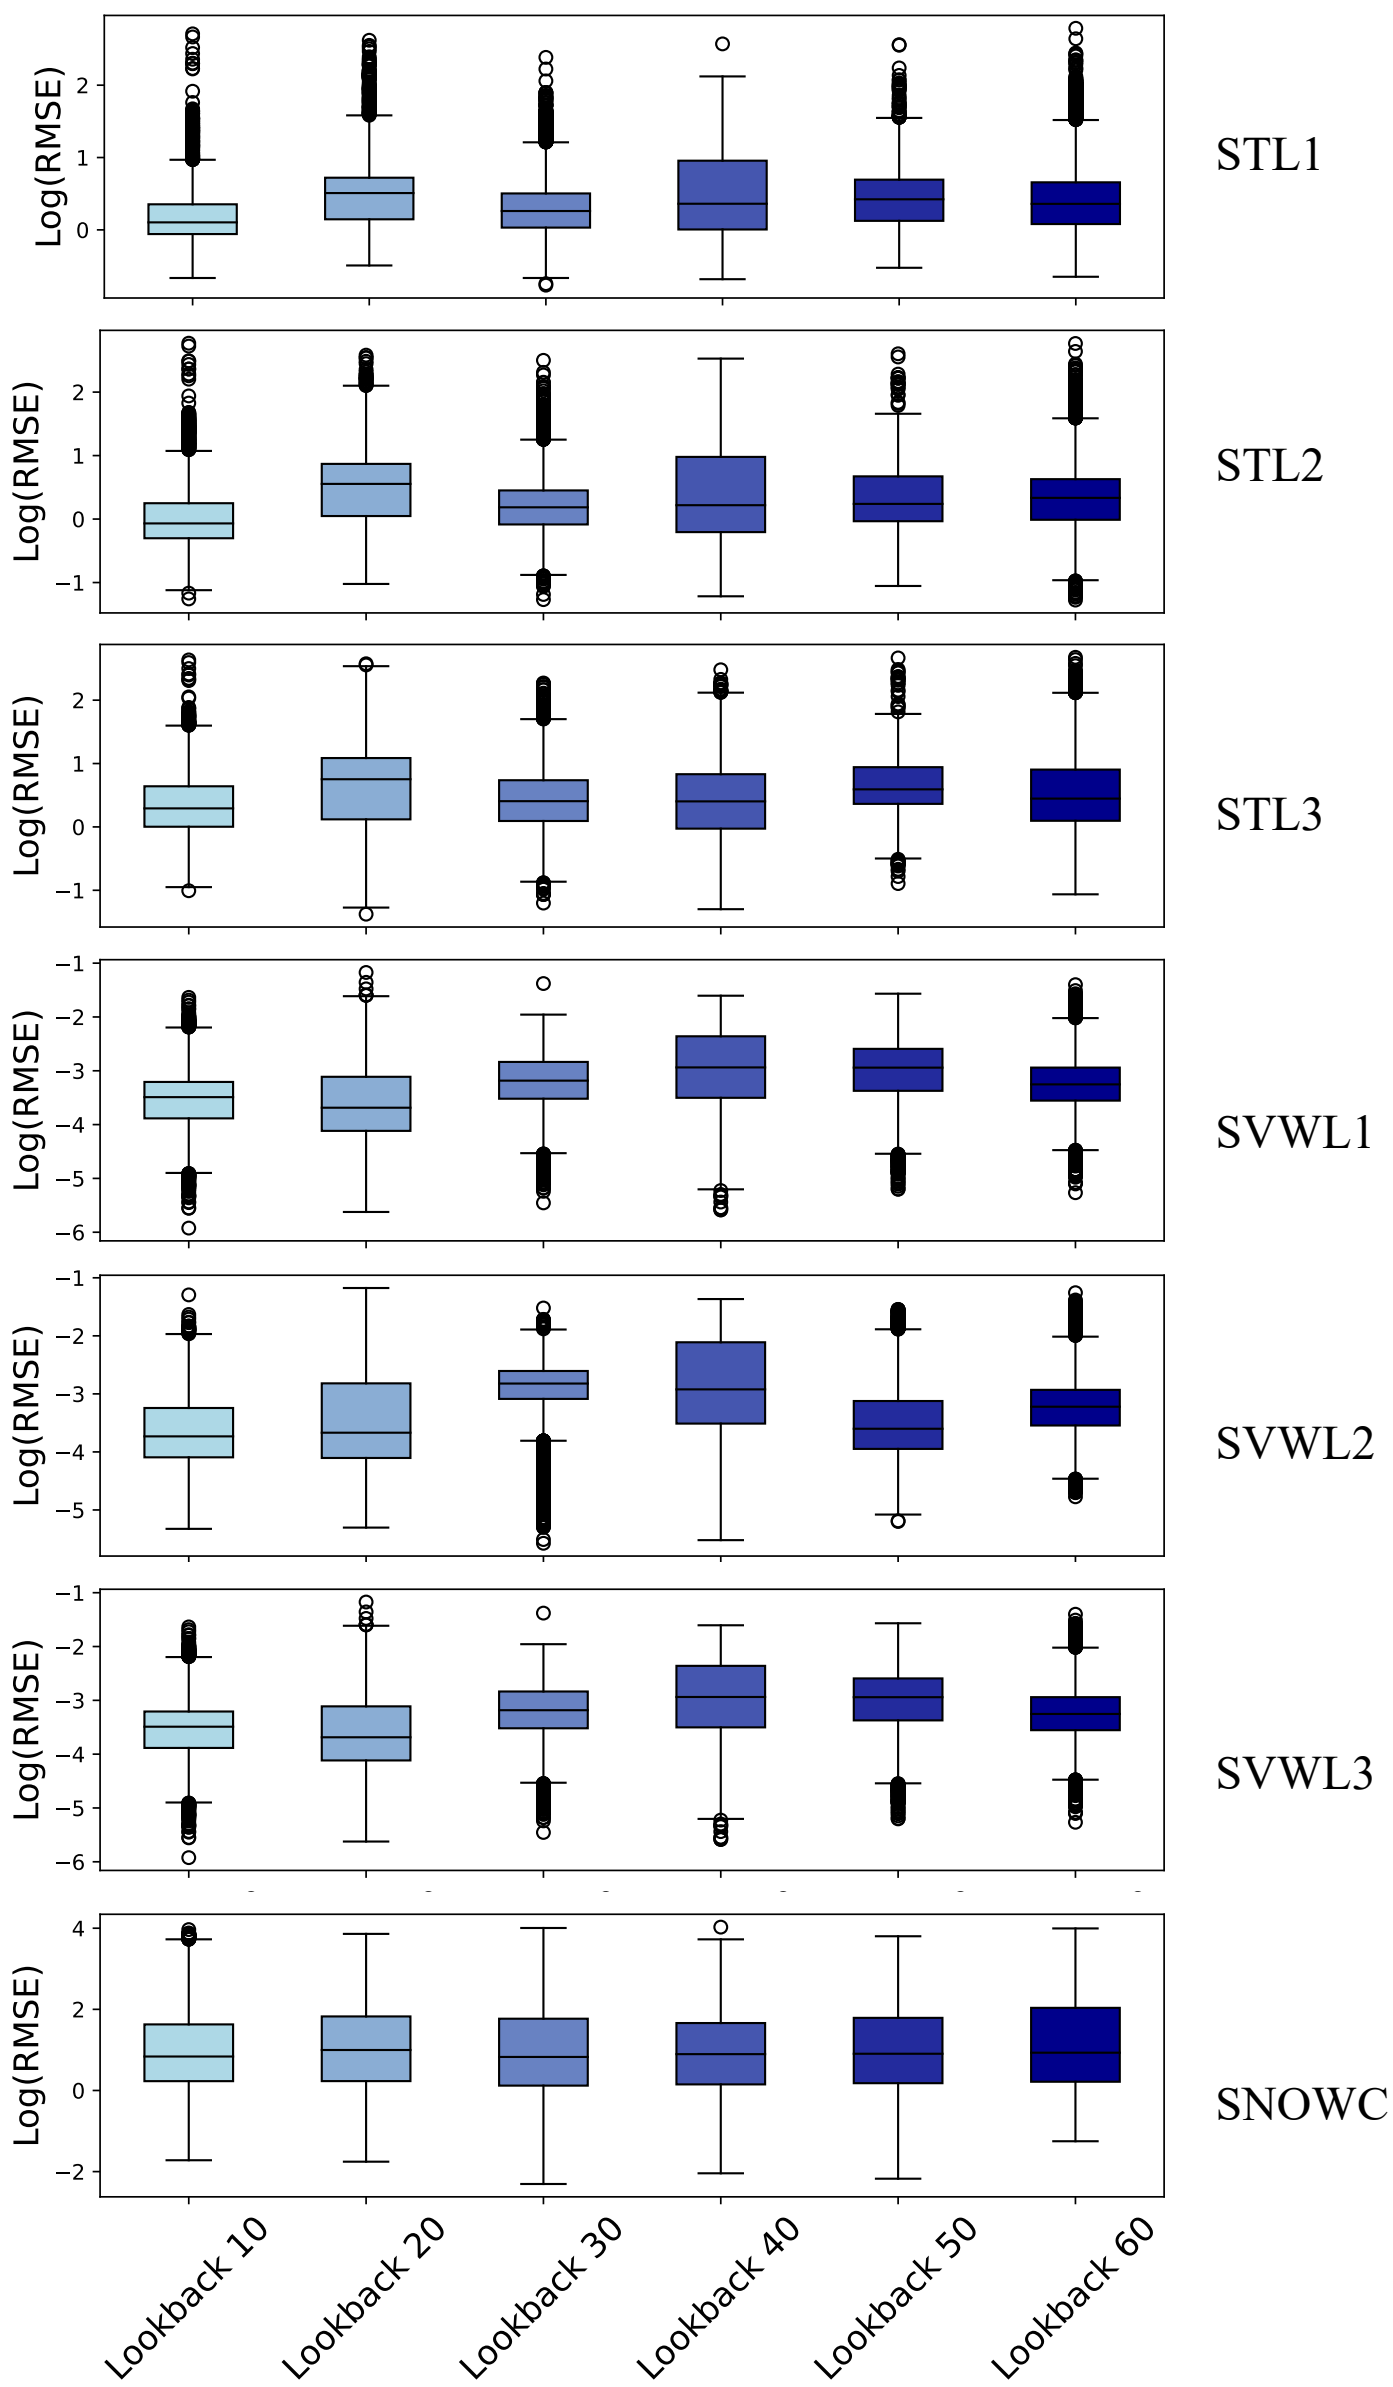

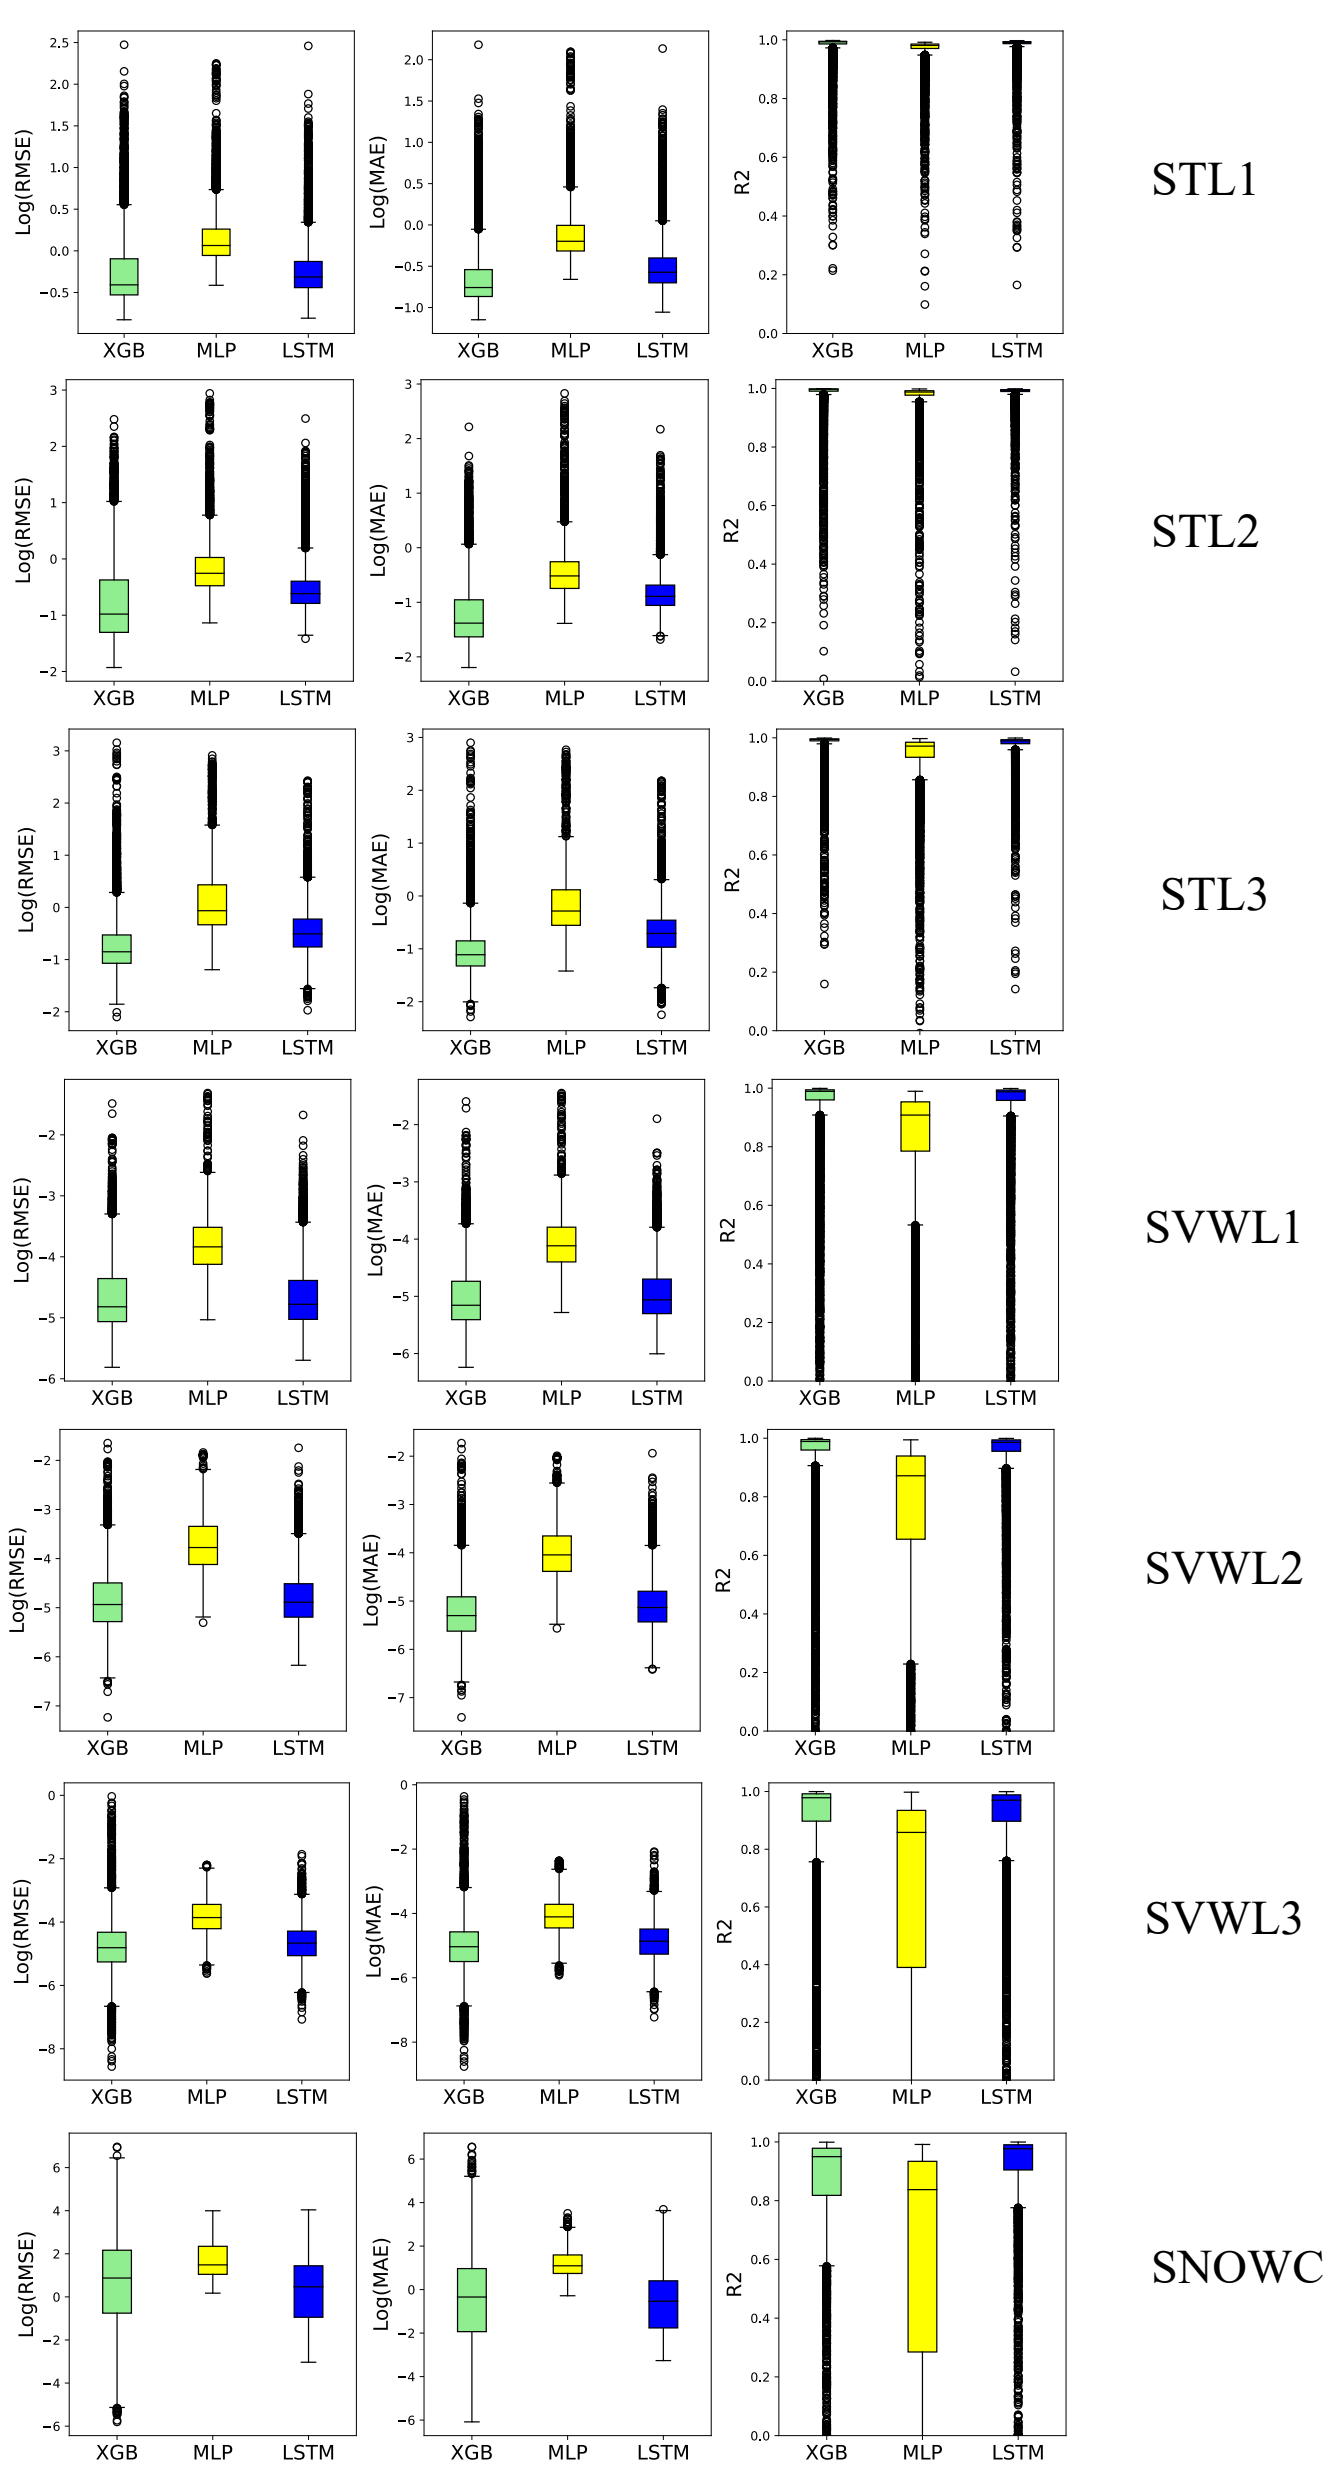

Supplement: Supplementary file 1 [file supp_fig03.pdf]
