# Supplementary material for: Advances in Land Surface Model-based Forecasting: A comparative study of LSTM, Gradient Boosting, and Feedforward Neural Network Models as prognostic state emulators
Source: arXiv:2407.16463 source file (2024-07-23)

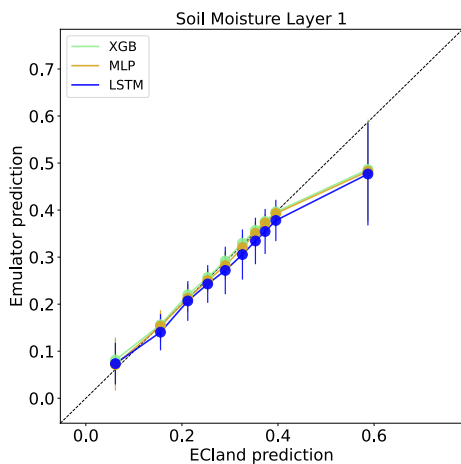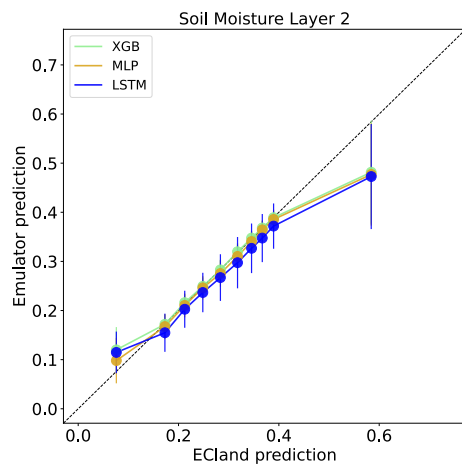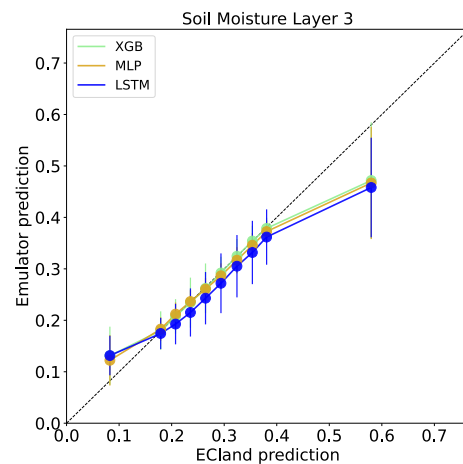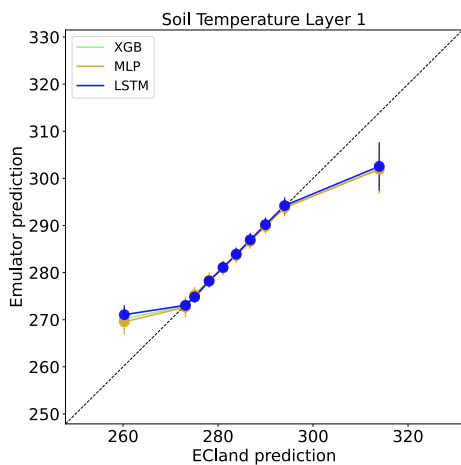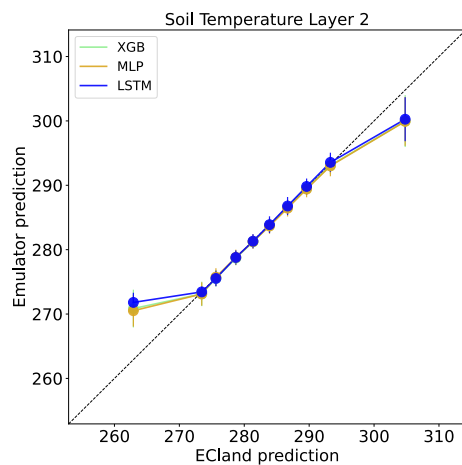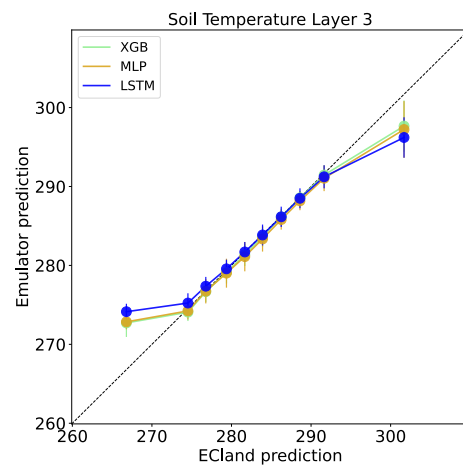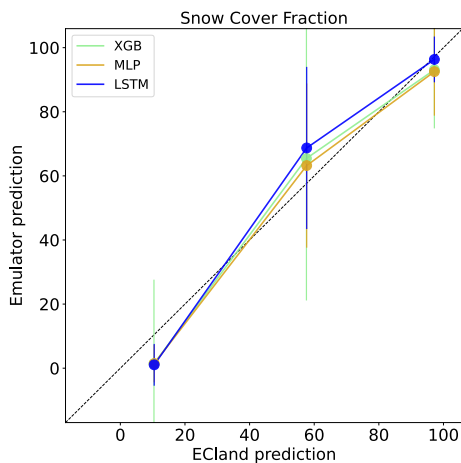

Soil Moisture Layer 1

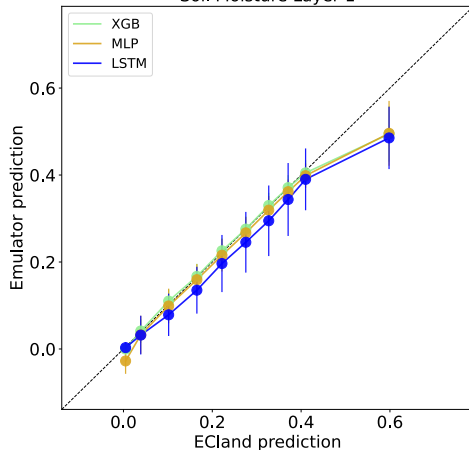

Soil Moisture Layer 2

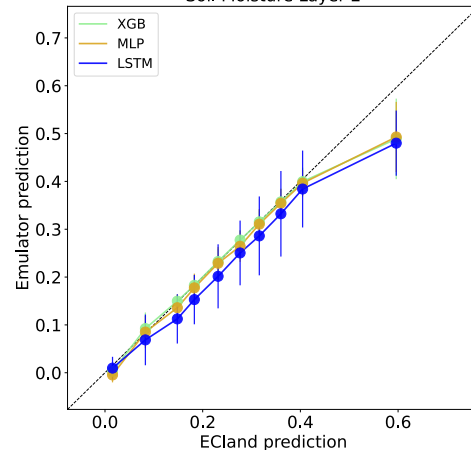

Soil Moisture Layer 3

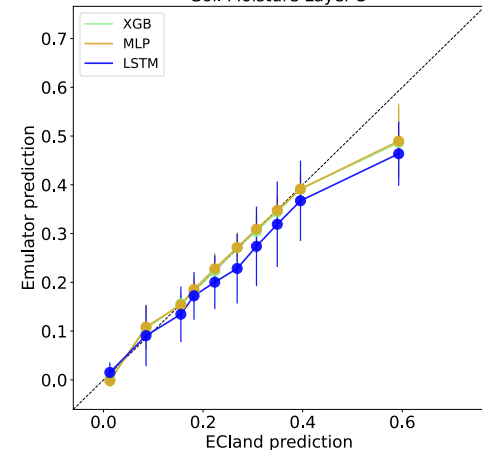

Soil Temperature Layer 1

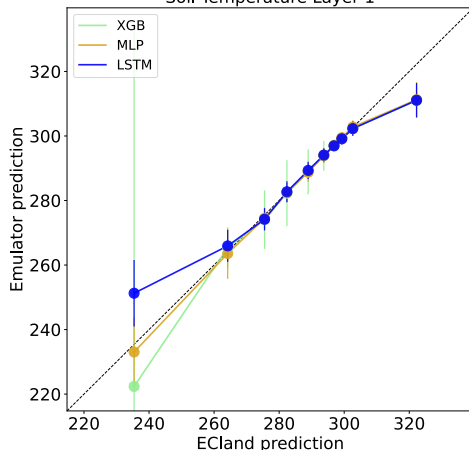

Soil Temperature Layer 2

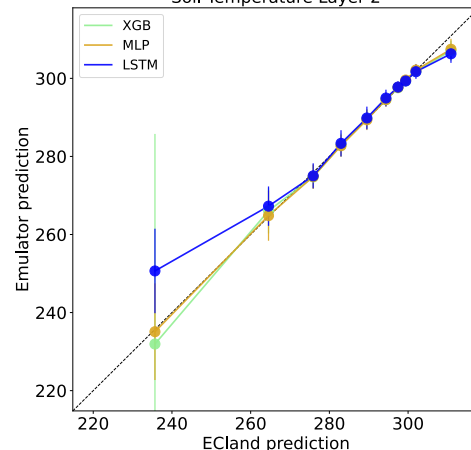

Soil Temperature Layer 3

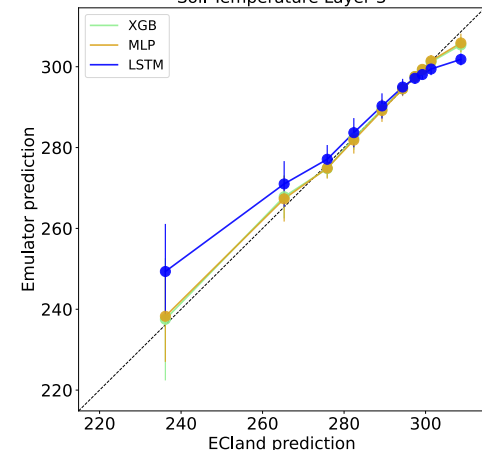

Snow Cover Fraction

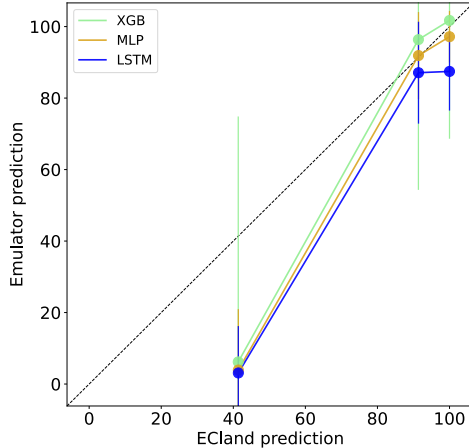

Supplement: Supplementary file 2 [file supp_fig07.pdf]
